# Supplementary material for: Distributed Resource Allocation with Multi-Agent Deep Reinforcement Learning for 5G-V2V Communication
Source: arXiv:2010.05290 source file (2020-10-11)
Supplement: Supplementary file 1 [file appendix.tex]

\appendix
\subsection{View-based positional distribution common knowledge}\label{sec:appendix_know}
In this appendix, we share the formulation of view-based common knowledge inspired from the paper \cite{DeWitt2018}. All vehicles have a circular field of view with a fixed radius(set based on communication range). Then, common knowledge $\mathcal{I}^{\mathcal{G}}$ between groups of $\mathcal{G}$ of agents arises through entity-based field-of-view common knowledge\cite{DeWitt2018}.

The state $s$ is composed of a number of entities $e\in \varepsilon$ with state features $s^e$ i.e. $s = \{s^e | e \in \varepsilon\}$. In this work, all entities are agents $a \in \mathcal{A} \equiv \varepsilon$ and $s^a$ is the position of vehicles i.e. $s^a = (x^a, y^a)$. The observation $z^a$ contains the subset of state features $s^e$ from all the entities $e$ that $a$ can see. Whether $a$ can see $e$ is determined by the binary mask $\mu^a(s^a, s^e)\in \{\bot, \top\}$. In our scenario, binary mask checks whether the distance between $s^a, s^e$ is lower than the observation radius $R$. Also, $\mu^a$ and $R$ are the same for all agents. The set of all entities the agent $a$ can see is therefore $\mathcal{M}^a := \{e | \mu^a(s^a, s^e)\} \subseteq \varepsilon$. The agent's observation is specified by the deterministic observation function $o(s,a)$ such that $z^a = o(s,a)=\{s^e | e \in \mathcal{M}^a\} \in \mathcal{Z}$. Then, each agent receives $z^a$ e.g. positions of the observed vehicles to create \textit{view-based positional distribution} vector such that $v^a = g(z^a, B, R)$. 

In our scenario, agents are homogeneous i.e. the function $g$, binary mask $\mu^a$ and variables $B, R$ are the same for all agents. Furthermore, our aim is to learn cooperative behavior in centralized training e.g. far vehicles should learn to select the same action/resource. Thus, the model can learn the common knowledge function $\mathcal{I}^{\mathcal{G}}$.

Then, the commonly known trajectory $\tau_t^G$;
\begin{equation}
    \tau_t^{\mathcal{G}} := \mathcal{I}^{\mathcal{G}}(\tau_t^a) = \mathcal{I}^{\mathcal{G}}(\tau_t^{\overline{a}}) , \forall a, \overline{a} \in \mathcal{G}.
\end{equation}
From the observation trajectory, $\tau_t^a = (v_1^a, ..., v_t^a)$ of any agent $a \in \mathcal{G}$. The commonly known position distribution $v_k^{\mathcal{G}} = \{g(z_k^{\mathcal{G}}, B, R) |z_k^{\mathcal{G}}\in \mathcal{Z}, B\in \mathbb{Z}^+, R\in \mathbb{Z}^+\}$ with $z_k^{\mathcal{G}} = \{s_k^e | e\in \mathcal{I}^{\mathcal{G}} \}$. The commonly known trajectory
\begin{equation}
\begin{split}
         \tau_t^{\mathcal{G}} = (v_1^{\mathcal{G}},\mathbf{u}_1^{\mathcal{G}},..., v_t^{\mathcal{G}},\mathbf{u}_t^{\mathcal{G}} ) \\
         \mathbf{u}_t^{\mathcal{G}} := (u_t^{a},..., u_t^{a}), a \in \mathcal{G} \\
         \text{with policy  } \pi^{\mathcal{G}}(u_t^{a}|\tau_{t}^{\mathcal{G}},\tau_t^a ).\\
\end{split}
\label{eq:commonknowledge}
\end{equation}

Each agent can deduce the commonly known positional distribution vector from its view-based positional distribution and individual action for each agent can be obtained by condition on commonly known positional distribution and view-based position distribution Equation \ref{eq:commonknowledge}. Simply, if all agents in the system can see each other, then an agent can estimate the observations of the others from its own observation and selects an action by estimating the actions of others to maximize the system objective. Each agent view is the group's joint view, joint actions are generated based on this joint view. Each agent performs its part from the joint action which is determined by the view of the agent.

In this work, actions of the agent do not change \textit{directly} the construction of common knowledge. Unless all use the same resource persistently for transmission, then agents can not receive the messages of others due to half-duplexity constraint. Then, agents remove the positions of other agents from their neighboring table if they can not receive any update for the last $m$ transmissions from other agents. Thus, the action of agent $a_t^{i}$ has only a long term effect on common knowledge. In this work, common knowledge mainly depends on the system dynamics i.e. mobility of vehicles. This can simplify the problem since learning system dynamics(LSTM helps for mobility prediction) easier than developing common knowledge. Otherwise, we would need to know the actions of other agents in order to take an individual action based on local observation or we would need to take joint actions as in \cite{DeWitt2018}. Then, we might say that relying on common knowledge which is deducted by the information that is \textit{not} directly affected by the actions of the agents, can improve cooperative behaviour and allow the model to develop individual actions instead of joint actions based on local observations. 

\subsection{Neighbor Table Updates} \label{app:neigh}
Each vehicle holds a neighboring table which includes the positions of the other vehicles on the road and piggybacks the neighboring table together with the CAM messages so that every vehicle on the road knows the positions of the other vehicles. We adopt a similar mechanism to keep the neighboring table updated as a destination-sequenced-distance vector(DSDV) routing scheme which is based on the Bellman-Ford algorithm \cite{10.1145/190314.190336}. Each entry in the neighbor table contains a sequence number along with vehicle id and positions, which is updated(increased by "1") by the vehicle of the entry for every transmitted CAM message. When a vehicle receives a CAM message from the other vehicles, it checks every entry in the neighbor table of the transmitter in the CAM message. If the sequence number in an entry of the transmitter neighbor table is higher than the sequence number of the same entry(indicates the same vehicles), the receiver updates the positions of the vehicle in the entry with the positions received by transmitter neighbor table.

Additionally, each entry in the table includes a \textit{last update} counter which expresses the time between the updates of this entry. When a vehicle piggybacks its neighbor table together with a CAM message, it increases the \textit{last update} counter in all the entries except its own entry. When a vehicle receives a neighbor table of the transmitter which has a higher sequence number for the same entry, it reset the \textit{last update} counter to zero. If the \textit{last update} counter is higher than a threshold which can be adjusted based on mobility e.g. 2 seconds, then we omit this entry when extracting positional distribution from the table assuming that the receiver vehicle is no longer in the coverage of the transmitter vehicle. Note that, we apply such a mechanism so that all vehicles on the road can know the updated positions of the other vehicles. We refer to the paper \cite{10.1145/190314.190336} for readers to get more intuitions about the mechanism.
